# Supplementary material for: Detecting Localized Adversarial Examples: A Generic Approach using Critical Region Analysis
Source: arXiv:2102.05241 source file (2021-02-14)
Supplement: Supplementary file 1 [file Appendix.tex]

% \clearpage
\begin{appendices}

\section{Details of Region Misleading Attacks}
\label{appendix:regionDetails}

The goal of the attack is to achieve misclassification and critical region misleading at the same time. To launch the attack, we formulate the following equation for optimization to get a patch $p$ that applies to image input $x$ with function $A$
\begin{equation}
\label{eq:regionMislead}
\min_{p} \left(1-\lambda\right)\ell_{\mathrm{prd}}\left(f(A(p,x)), c_{t}\right)+\lambda \ell_{\mathrm{est}}\left(e(A(p,x) ; f), g_{t}\right),
\end{equation}
where $\ell_{\mathrm{prd}}$ is the prediction loss between the current state $f(A(p, x))$ and target $c_{t}$, and $\ell_{\mathrm{est}}$ is the distance between the estimated area $e(x ; f)$ and the ground truth adversarial region $g_{t}$. Under this setting, we define $\ell_{\text {est }}\left(e(A(p, x) ; f), g_{t}\right)=-\| e(A(p, x) ; f)- g_{t} \|_{p}$ with a negative sign to maximize the distance. An example of the misleading attack with a low IoU score is shown in Figure~\ref{fig:misleadExample}, which shows that \name{} is robust to locate the attack even after a strong misleading.

\begin{figure}[h]

 	\centering
	
 	\subfloat[]{
 		\begin{minipage}[t]{0.3\linewidth}
 			\centering
 			\includegraphics[width=0.9in]{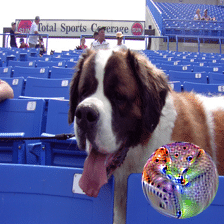}
 			%\caption{fig1}
 		\end{minipage}%
 	}%
 	\subfloat[]{
 		\begin{minipage}[t]{0.3\linewidth}
 			\centering
 			\includegraphics[width=0.9in]{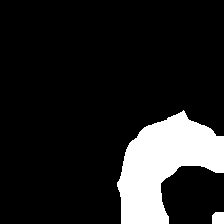}
 			%\caption{fig2}
 		\end{minipage}%
 	}%
 	\subfloat[]{
 	\begin{minipage}[t]{0.3\linewidth}
 		\centering
 		\includegraphics[width=0.9in]{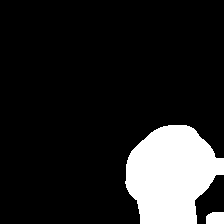}
 		%\caption{fig2}
 	\end{minipage}%
 	}%
	
 	\subfloat[]{
 	\begin{minipage}[t]{0.3\linewidth}
 		\centering
 		\includegraphics[width=0.9in]{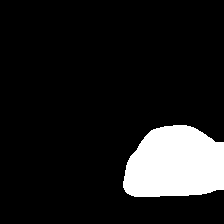}
 		%\caption{fig2}
 	\end{minipage}%
 	}%
 	\subfloat[]{
 	\begin{minipage}[t]{0.3\linewidth}
 		\centering
 		\includegraphics[width=0.9in]{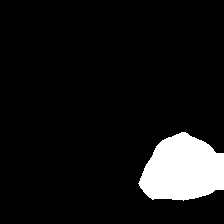}
 		%\caption{fig2}
 	\end{minipage}%
 	}%
 	\subfloat[]{
 	\begin{minipage}[t]{0.3\linewidth}
 		\centering
 		\includegraphics[width=0.9in]{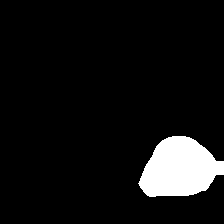}
 		%\caption{fig2}
 	\end{minipage}%
 	}%

  	\centering
  	\caption{The behavior of \name{} under the region misleading attack. (a) shows the victim image and (b) is the region estimation. (c), (d) and (e) are three examples of the sub-masks. (f) is the final region we obtain.}
    \label{fig:misleadExample}
\end{figure}

Moreover, there exists other attack options, such as region minimization or misleading region estimation to a predefined area (i.e., region targeting attack). With the same experimental settings, we evaluate \name{} against these attacks. For region minimization attack, we define $\ell_{\text {est }}\left(e(A(p, x) ; f), g_{t}\right)=\| e(A(p, x) ; f) * g_{t} \|_{p}$. For region targeting attack, we set $\ell_{\text {est }}$ as $\| e(A(p, x) ; f) - tar_{t} \|_{p}$, where $tar_{t}$ is the target region. The result is shown in Figure~\ref{fig:misleadAdditional}, the attack success rates with \name{} under different settings are all below 10\%. Note that, we only show results of $l_{est}$ using $l_{2}$ distance here, while it exhibits nearly identical results when using $l_{1}$ and $l_{2}$ distances.

\section{Performance under Different FPR Settings}
\label{appendix:deltailPerformance}
To further illustrate the detailed effectiveness apart from results shown in Section \ref{sec:Experiments}, we include a detailed performance on the scene classification task in Tabel \ref{table:fpr3} when setting FPR as 3\%, the generated parameters are 9 and 5 for K and $\Delta R$, respectively. The detailed results with respect to different FPR settings on the face recognition task are already shown in Fig. \ref{fig:TPR_glasses}.

\begin{figure*}[t]
    \vspace*{-9cm}
	\centering 
	%\vspace{1cm}
	\subfloat[Minimization attack]{
	    \includegraphics[width=0.4\linewidth]{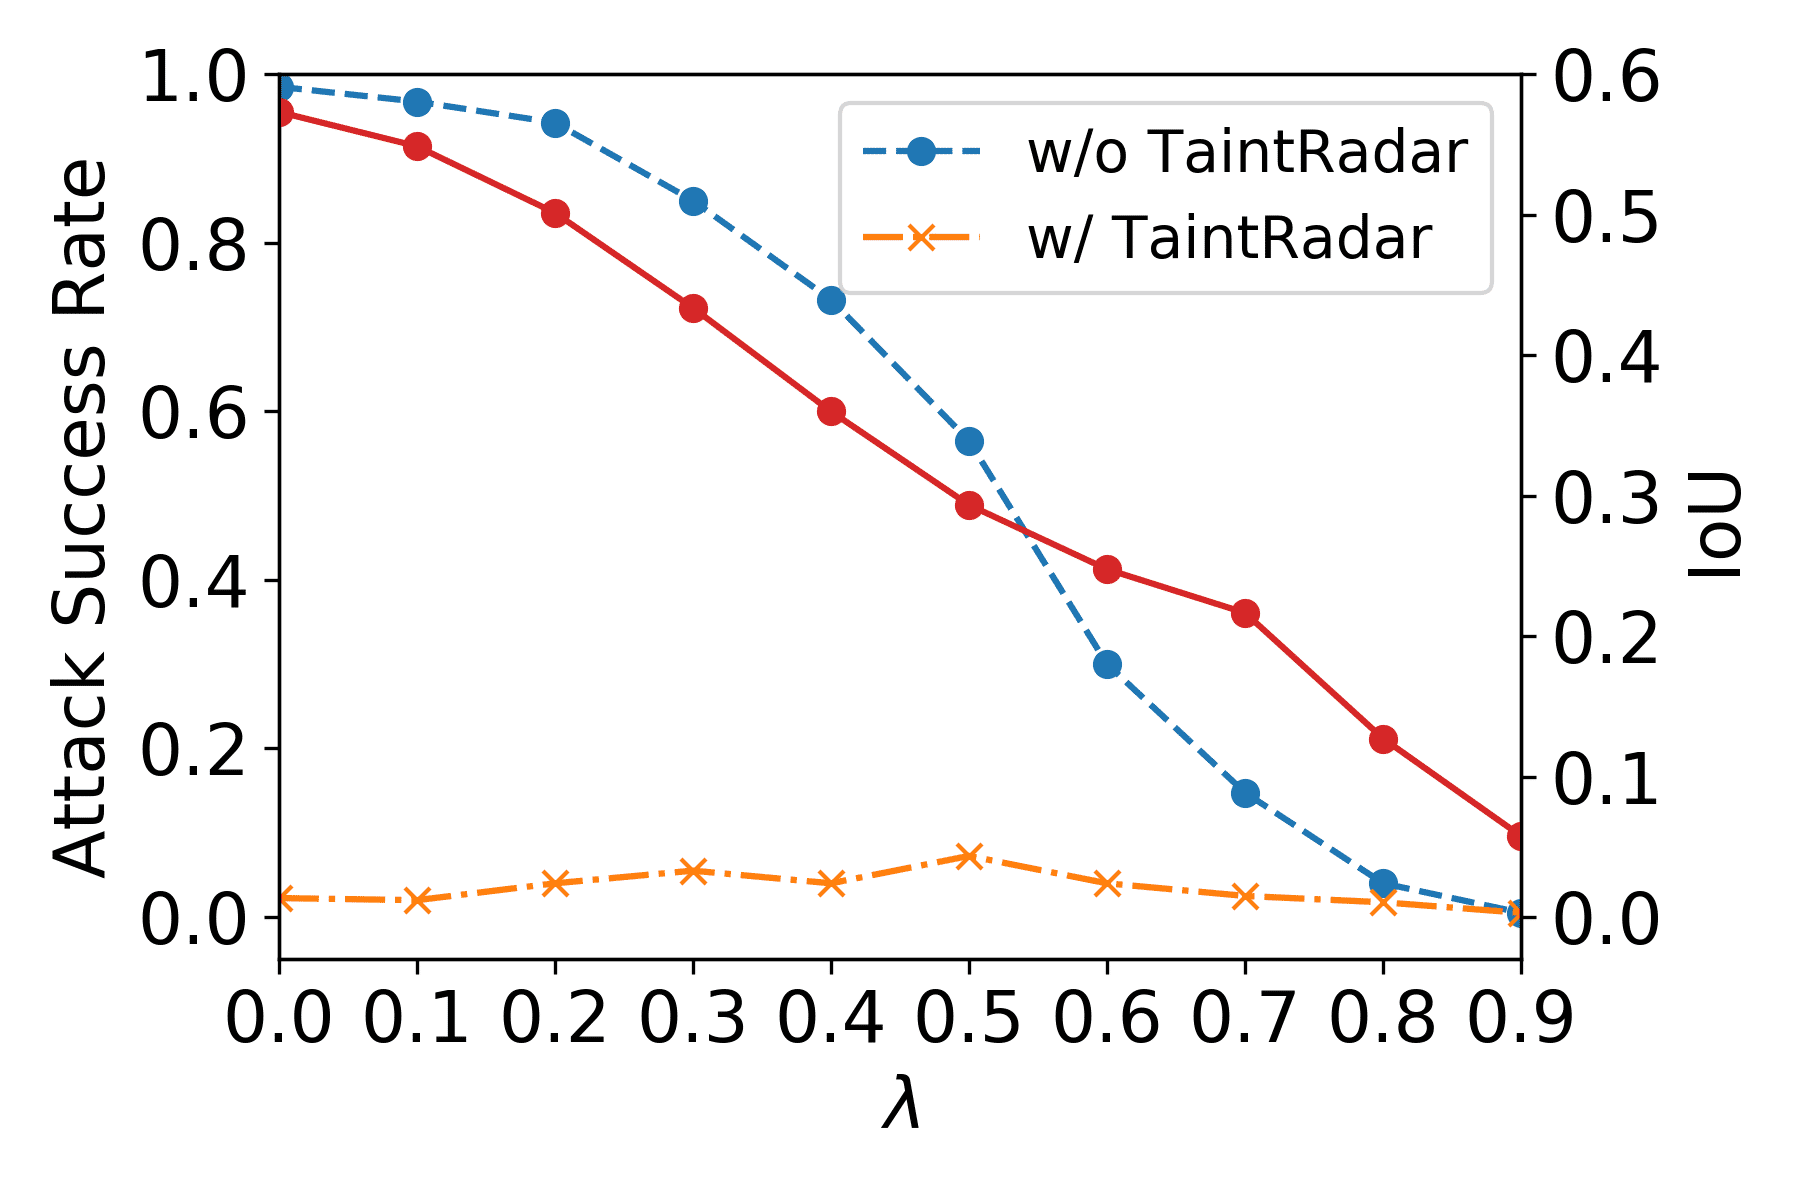}
	}
	\subfloat[Region targeting attack]{
	    \includegraphics[width=0.4\linewidth]{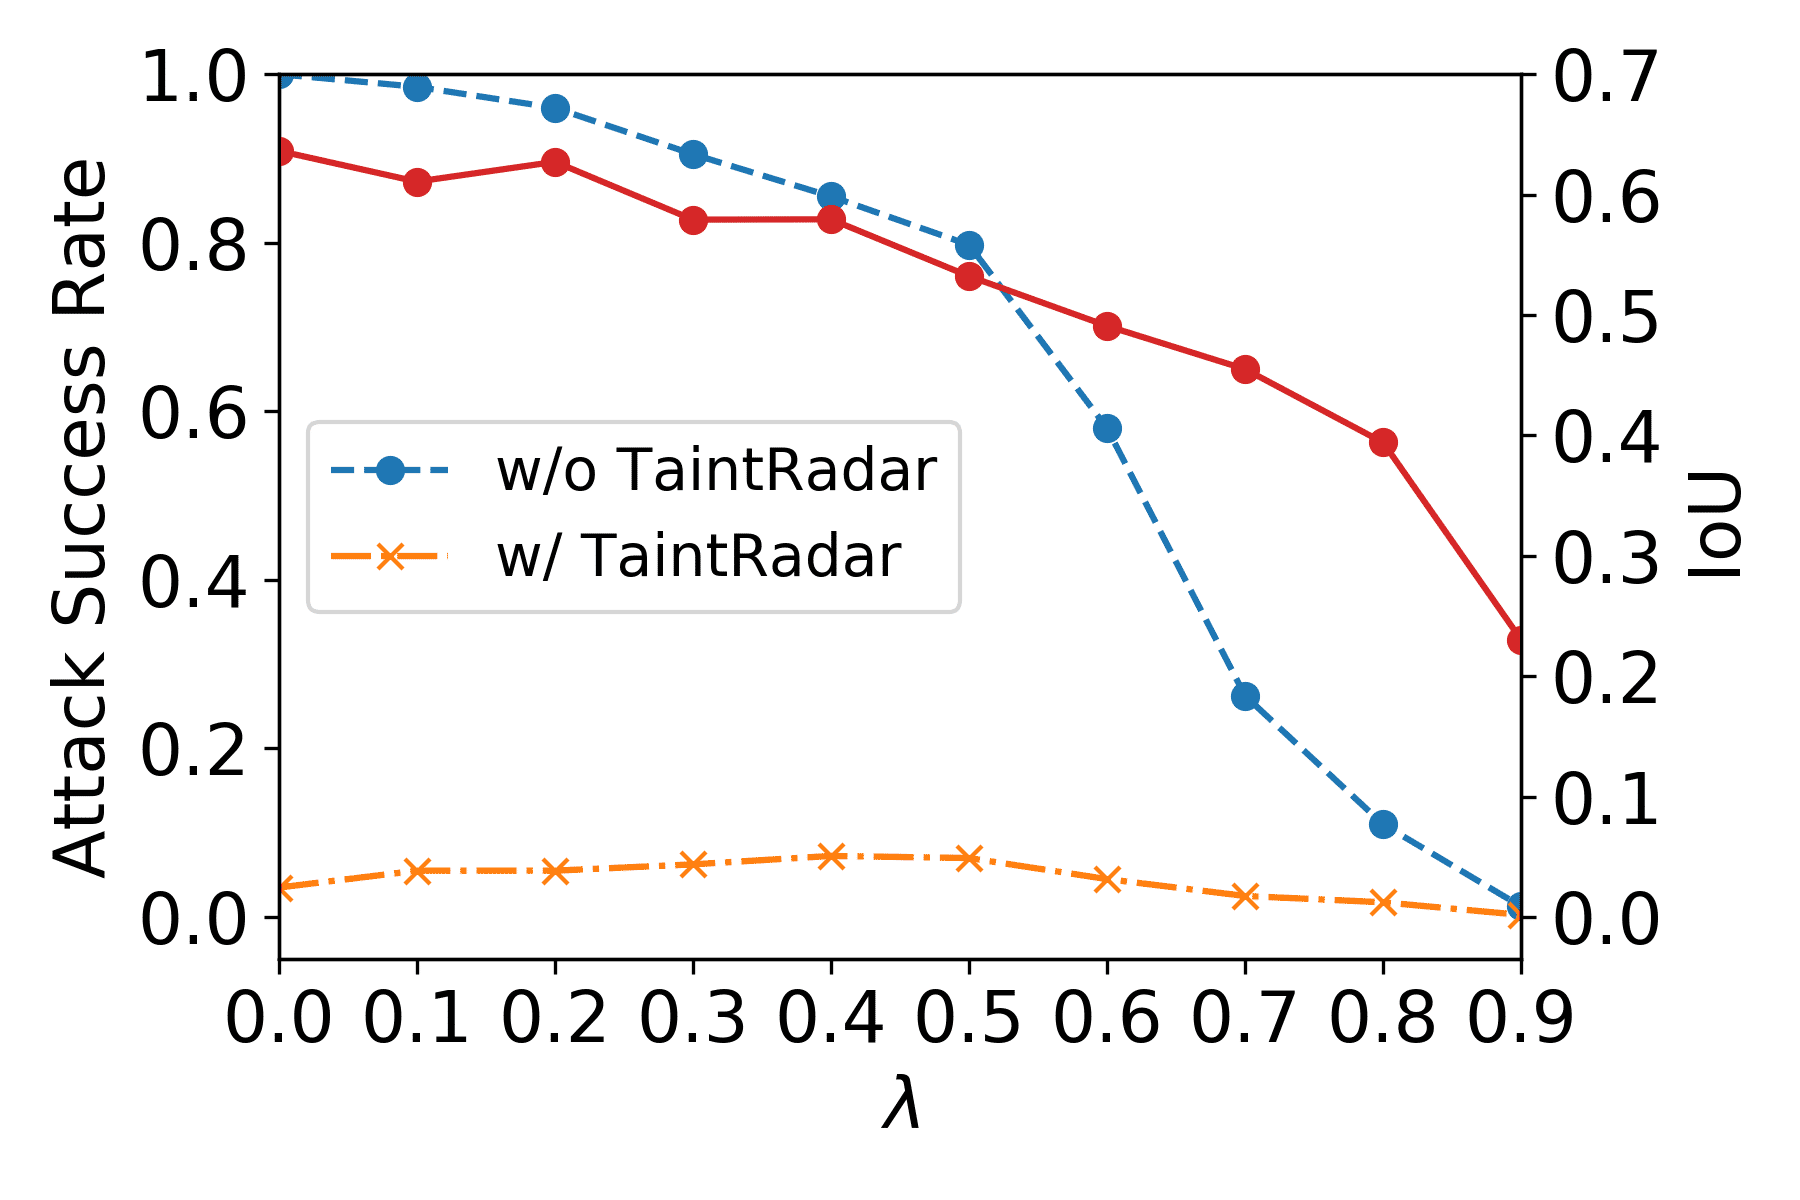}
	}
	
	\caption{The impact of region minimization and targeting attacks on \name{}. The solid line shows the averaged IoU value of generated attacks, and the dashed lines represent the attack success rates with or without \name{}.}
	\label{fig:misleadAdditional}
% 	\label{fig:regionMislead}
\end{figure*}

\begin{table*}[t]
\vspace*{-19cm}
\caption{3\% FPR. The results on TPR against adversarial patches and the final success rate after (SR) under four different variables. SR is calculated based on the successfully-generated rate and the detection rate.}
\label{table:fpr3}
\resizebox{\textwidth}{!}{ 
\begin{tabular}{cc|cc|cc|cc|cc|cc|cc}
\toprule[1.5pt]
 &  & \multicolumn{6}{c|}{\textbf{Single Size}} & \multicolumn{6}{c}{\textbf{Multiple Sizes}} \\ \midrule[1.5pt]
 & \multicolumn{1}{|c|}{\textbf{Batch Size}} & \multicolumn{2}{c|}{1} & \multicolumn{2}{c|}{4} & \multicolumn{2}{c|}{16} & \multicolumn{2}{c|}{1} & \multicolumn{2}{c|}{4} & \multicolumn{2}{c}{16} \\
 \cline{2-14}
\textbf{Position} & \multicolumn{1}{|c|}{\textbf{Patch Size}} & TPR & SR & TPR & SR & TPR & \multicolumn{1}{c|}{SR} & TPR & SR & TPR & SR & TPR & SR \\ \hline
\multicolumn{1}{c|}{\multirow{3}{*}{\textbf{\begin{tabular}[c]{@{}c@{}}Right-\\ bottom\end{tabular}}}} & 0.2 & 97.96\% & 0.75\% & 98.17\% & 0.50\% & 97.37\% &  \multicolumn{1}{c|}{0.75\%} & 80.00\% & 1.25\% & 94.74\% & 0.25\% & 91.67 \% & 0.5\% \\
\multicolumn{1}{c|}{} & 0.3 & 97.70\% & 2.25\% & 98.43\% & 1.50\% & 97.94\% & \multicolumn{1}{c|}{2.00\%} & 95.51\% & 3.50\% & 98.45\% & 1.25\% & 94.88\% & 4.25\% \\
\multicolumn{1}{c|}{} & 0.4 & 89.75\% & 10.25\% & 96.48\% & 3.50\% & 96.50\% & \multicolumn{1}{c|}{3.50\%} & 84.90\% & 14.50\% & 91.58\% & 8.25\% & 85.71\% & 14.00\% \\ %\cline{1-14} 
\hline
\multicolumn{1}{c|}{\multirow{3}{*}{\textbf{Random}}} & 0.2 & 94.83\% & 3.00\% & 95.18\% & 1.75\% & 95.45\% & \multicolumn{1}{c|}{2.00\%} & 77.42\% & 3.50\% & 91.30\% & 1.00\% & 79.59\% & 2.50\% \\
\multicolumn{1}{c|}{} & 0.3 & 94.94\% & 5.00\% & 98.00\% & 2.00\% & 94.33\% & \multicolumn{1}{c|}{5.50\%} & 91.55\% & 7.25\% & 94.68\% & 4.75\% & 93.71\% & 5.75\% \\
\multicolumn{1}{c|}{} & 0.4 & 84.25\% & 15.75\% & 94.25\% & 5.75\% & 88.47\% & \multicolumn{1}{c|}{11.50\%} & 77.49\% & 22.00\% & 84.89\% & 15.00\% & 77.00\% & 22.75\% \\ 
\bottomrule[1.5pt]
\end{tabular}
}
\end{table*}

\end{appendices}
